# Supplementary material for: LOKI: A Comprehensive Synthetic Data Detection Benchmark using Large Multimodal Models
Source: arXiv:2410.09732 source file (2025-04-21)
Supplement: Supplementary file 1 [file sec7_supp.tex]

\textbf{Image:} We collected a variety of image types. The paired synthetic and real data for general images were sourced from the internet and datasets like I2IQA, Sentry, GenImage, and FFHQ. Remote sensing images were based on the CVUSA and VIGOR datasets and synthesized using GAN or Diffusion methods, covering both urban and suburban scenes. Medical images included tumor images from the M3DSynth dataset and newly synthesized skin disease images from the ISBI 2016 dataset. Document images were synthesized using layout generation and rule-based algorithms, covering four categories: newspaper, paper, magazine, and reconstruction, with ground truth data sourced from the M6Doc dataset.

\raggedright
\begin{itemize}
    \item \textbf{GPT-4o} (\texttt{gpt-4o-2024-08-06}): \url{https://platform.openai.com/docs/models/gpt-4o}
    \item \textbf{Gemini-1.5-Flash} (\texttt{gemini-1.5-flash}): \url{https://ai.google.dev/gemini-api/docs/models/gemini}
    \item \textbf{Claude-3.5-Sonnet} (\texttt{claude-3-5-sonnet-20240620}): \url{https://docs.anthropic.com/en/docs/about-claude/models}
    \item \textbf{Mistral} (\texttt{mistral-large-latest}): \url{https://docs.mistral.ai/getting-started/models/}
    \item \textbf{Qwen-Max} (\texttt{qwen-max}): \url{https://www.alibabacloud.com/help/en/model-studio/developer-reference/use-qwen-by-calling-api}
\end{itemize}

\raggedright
\begin{itemize}
    \item \textbf{InternVL2-8B} (\texttt{OpenGVLab/InternVL2-8B}): \url{https://huggingface.co/OpenGVLab/InternVL2-8B}
    \item \textbf{InternVL2-40B} (\texttt{OpenGVLab/InternVL2-40B}): \url{https://huggingface.co/OpenGVLab/InternVL2-40B}
    \item \textbf{InternVL2-Llama3-76B} (\texttt{OpenGVLab/InternVL2-Llama3-76B}): \url{https://huggingface.co/OpenGVLab/InternVL2-Llama3-76B}
    \item \textbf{LLaVA-OneVision-7B} (\texttt{lmms-lab/llava-onevision-qwen2-7b-ov}): \url{https://huggingface.co/lmms-lab/llava-onevision-qwen2-7b-ov}
    \item \textbf{LLaVA-OneVision-72B} (\texttt{lmms-lab/llava-onevision-qwen2-72b-ov-sft}): \url{https://huggingface.co/lmms-lab/llava-onevision-qwen2-72b-ov-sft}
    \item \textbf{VILA-1.5-13B} (\texttt{Efficient-Large-Model/VILA1.5-13b}): \url{https://huggingface.co/Efficient-Large-Model/VILA1.5-13b}
    \item \textbf{VILA-1.5-40B} (\texttt{Efficient-Large-Model/VILA1.5-40b}): \url{https://huggingface.co/Efficient-Large-Model/VILA1.5-40b}
    \item \textbf{Phi-3.5-Vision} (\texttt{microsoft/Phi-3.5-vision-instruct}): \url{https://huggingface.co/microsoft/Phi-3.5-vision-instruct}
    \item \textbf{idefics2-8b} (\texttt{HuggingFaceM4/idefics2-8b}): \url{https://huggingface.co/HuggingFaceM4/idefics2-8b}
    \item \textbf{Qwen2-VL-7B} (\texttt{Qwen/Qwen2-VL-7B-Instruct}): \url{https://huggingface.co/Qwen/Qwen2-VL-7B-Instruct}
    \item \textbf{Qwen2-VL-72B} (\texttt{Qwen/Qwen2-VL-72B-Instruct}): \url{https://huggingface.co/Qwen/Qwen2-VL-72B-Instruct}
    \item \textbf{InternLM-XComposer-2d5} (\texttt{internlm/internlm-xcomposer2d5-7b}): \url{https://huggingface.co/internlm/internlm-xcomposer2d5-7b}
    \item \textbf{mplug-owl3} (\texttt{mPLUG/mPLUG-Owl3-7B-240728}): \url{https://huggingface.co/mPLUG/mPLUG-Owl3-7B-240728}
    \item \textbf{MiniCPM-V2.6} (\texttt{openbmb/MiniCPM-V-2\_6}): \url{https://huggingface.co/openbmb/MiniCPM-V-2_6}
    \item \textbf{LongVILA} (\texttt{Efficient-Large-Model/Llama-3-LongVILA-8B-128Frames}): \url{https://huggingface.co/Efficient-Large-Model/Llama-3-LongVILA-8B-128Frames}
    \item \textbf{LongVA-7B} (\texttt{lmms-lab/LongVA-7B-DPO}): \url{https://huggingface.co/lmms-lab/LongVA-7B-DPO}
\end{itemize}

\begin{table}[ht]
\centering
\caption{Synthetic Methods Across Modalities}
\begin{tabular}{c c}
\toprule
\textbf{Modality} & \textbf{Synthesis Method} \\ 
\midrule
Video & \makecell{Sora, Keling, CoNo, LaVie, Open-sora, \\ Runway, W.A.L.T} \\ 
\midrule
Image & \makecell{Stable Diffusion (V1.4,V1.5,V2.1), Midjourney, \\ FLUX, DDIM, DPM+, Euler, CZLCM, \\ ADM, Stylegan, Skydiffusion, pix2pix, CUT} \\ 
\midrule
3D & \makecell{CLAY, SyncDreamer, Magic3D, \\ DreamFusion, Fantasia3D, DreamGaussian, \\ Wonder3D, GaussianDreamer, GradeADreamer} \\ 
\midrule
Audio & \makecell{Suno, WaveNet, WaveRNN, Tacotron2, \\ Hifi-GAN, AceSinger, Soft-VITS-SVC, DiffSinger, \\ VQ-VAE, AudioLDM, VITS, AudioLDM2, MusicGen } \\ 
\midrule
Text & \makecell{GPT-4, Gemini, Qwen-2} \\ 
\bottomrule
\end{tabular}
\end{table}

\begin{table}[ht]
\centering
\caption{Repurposed Datasets Across Modalities}
\begin{tabular}{c c}
\toprule
\textbf{Modality} & \textbf{Datasets} \\ 
\midrule
Image & \makecell{I2IQA, Sentry, GenImage, \\ FFHQ, Stylegan3, Deepfakeface \\ ISBI 2016, M3DSynth, \\ M6Doc, CVUSA, VIGOR} \\ 
\midrule
3D & \makecell{OmniObject3D, GPTEval3D} \\ 
\midrule
Audio & \makecell{ASVSpoof2019, CtrSVDD, \\ DCASE2023 Track 7, MusicCaps}
 \\ 
\midrule
Text & GPT-4, Gemini, Qwen-2(6) \\ 
\bottomrule
\end{tabular}
\end{table}

\begin{table*}[!b]
\centering
\small
\begin{adjustbox}{scale = 0.8}
\begin{tabular}{@{}lccccccc@{}}
\toprule
\textbf{} & \textbf{Sora} & \textbf{Keling} & \textbf{CogVideoX} & \textbf{Lumiere} & \textbf{Open-sora} & \textbf{Runway} & \textbf{W.A.L.T} \\
 & (150) & (2,426) & (345) & (603) & (565) & (505) & (408)\\ \midrule

\color{Gray} Random Choice & \color{Gray} 18.0 & \color{Gray} 21.6 & \color{Gray} 18.3 & \color{Gray} 18.6 & \color{Gray} 26.0 & \color{Gray} 22.2 & \color{Gray} 22.1\\ 
\color{Gray} Frequent Choice & \color{Gray} 27.3 & \color{Gray} 24.0 & \color{Gray} 25.8 & \color{Gray} 19.9 & \color{Gray} 26.9 & \color{Gray} 26.1 & \color{Gray} 22.1\\
Expert (Worst)  & 78.0 & - & - & - & - & - & - \\
Expert (Medium)  & 84.7 & - & - & - & - & - & - \\
Expert (Best)  & 90.0 & - & - & - & - & - & - \\
\midrule
OpenFlamingo2-9B \cite{awadalla2023openflamingo} & 23.3 & 26.3 & 27.8 & 22.9 & 30.8 & 25.1 & 25.0 \\
Kosmos2 \cite{peng2023kosmos} & 19.3 & 26.6 & 28.4 & 21.7 & 29.2 & 26.7 & 28.4 \\
Fuyu-8B~\cite{fuyu-8b} & 22.0 & 25.6 & 27.8 & 20.9 & 30.1 & 24.8 & 25.7 \\
MiniGPT4-Vicuna-13B~\cite{zhu2023minigpt} & 28.7 & 26.2 & 23.2 & 22.1 & 29.4 & 30.1 & 25.5 \\
LLaMA-Adapter2-7B~\cite{zhang2023llama} & 30.7 & 25.6 & 27.5 & 24.9 & 30.4 & 23.0 & 21.3 \\
Otter~\cite{li2023otter} & 34.7 & 24.1 & 24.6 & 23.4 & 27.1 & 23.0 & 21.8 \\
CogVLM~\cite{COGVLM} & 28.0 & 25.1 & 29.3 & 24.2 & 28.0 & 23.4 & 21.1 \\
InstructBLIP-T5-XL~\cite{dai2023instructblip} & 32.7 & 25.2 & 27.0 & 22.1 & 28.3 & 24.4 & 25.0 \\
BLIP-2 FLAN-T5-XL \cite{li2023blip} & 30.7 & 25.1 & 26.7 & 24.4 & 25.7 & 24.0 & 25.2 \\
mPLUG-OWL2* \cite{ye2023mplug2} & 22.7 & 24.9 & 27.2 & 23.9 & 29.7 & 18.8 & 25.2 \\
SPHINX* \cite{lin2023sphinx} & 26.7 & 25.3 & 29.0 & 20.1 & 32.6 & 23.8 & 21.8  \\
Qwen-VL-7B-Chat~\cite{Qwen-VL} & 29.3 & 25.6 & 27.8 & 23.1 & 28.8 & 24.6 & 24.3 \\
Bunny-3B* \cite{Bunny-3B} & 30.7 & 26.8 & 32.8 & 25.2 & 27.8 & 26.5 & 22.8 \\
LLaVA-1.5-13B~\cite{liu2023improved} & 29.3 & 25.9 & 27.2 & 25.0 & 28.8 & 24.0 & 24.5 \\
\bottomrule
\end{tabular}%
\end{adjustbox}
\caption{\textbf{Science} results of different models on the \dataset \textbf{validation} and \textbf{test set}.  The best-performing model in each category is \textbf{in-bold}, and the second best is {\ul{underlined}}. *: results provided by the authors.} 
\label{tab:overall_Science_results}
\end{table*}

\begin{table*}[!b]
\centering
\small
\begin{adjustbox}{scale = 0.8}
\begin{tabular}{@{}lccccccc@{}}
\toprule
\textbf{} & \textbf{Sora} & \textbf{Keling} & \textbf{CogVideoX} & \textbf{Lumiere} & \textbf{Open-sora} & \textbf{Runway} & \textbf{W.A.L.T} \\
 & (150) & (2,426) & (345) & (603) & (565) & (505) & (408)\\ \midrule
\color{Gray} Random Choice & \color{Gray} 18.0 & \color{Gray} 21.6 & \color{Gray} 18.3 & \color{Gray} 18.6 & \color{Gray} 26.0 & \color{Gray} 22.2 & \color{Gray} 22.1\\ 
\color{Gray} Frequent Choice & \color{Gray} 27.3 & \color{Gray} 24.0 & \color{Gray} 25.8 & \color{Gray} 19.9 & \color{Gray} 26.9 & \color{Gray} 26.1 & \color{Gray} 22.1\\
Expert (Worst)  & 78.0 & - & - & - & - & - & - \\
Expert (Medium)  & 84.7 & - & - & - & - & - & - \\
Expert (Best)  & 90.0 & - & - & - & - & - & - \\
\midrule
OpenFlamingo2-9B \cite{awadalla2023openflamingo} & 23.3 & 26.3 & 27.8 & 22.9 & 30.8 & 25.1 & 25.0 \\
Kosmos2 \cite{peng2023kosmos} & 19.3 & 26.6 & 28.4 & 21.7 & 29.2 & 26.7 & 28.4 \\
Fuyu-8B~\cite{fuyu-8b} & 22.0 & 25.6 & 27.8 & 20.9 & 30.1 & 24.8 & 25.7 \\
MiniGPT4-Vicuna-13B~\cite{zhu2023minigpt} & 28.7 & 26.2 & 23.2 & 22.1 & 29.4 & 30.1 & 25.5 \\
LLaMA-Adapter2-7B~\cite{zhang2023llama} & 30.7 & 25.6 & 27.5 & 24.9 & 30.4 & 23.0 & 21.3 \\
Otter~\cite{li2023otter} & 34.7 & 24.1 & 24.6 & 23.4 & 27.1 & 23.0 & 21.8 \\
CogVLM~\cite{COGVLM} & 28.0 & 25.1 & 29.3 & 24.2 & 28.0 & 23.4 & 21.1 \\
InstructBLIP-T5-XL~\cite{dai2023instructblip} & 32.7 & 25.2 & 27.0 & 22.1 & 28.3 & 24.4 & 25.0 \\
BLIP-2 FLAN-T5-XL \cite{li2023blip} & 30.7 & 25.1 & 26.7 & 24.4 & 25.7 & 24.0 & 25.2 \\
mPLUG-OWL2* \cite{ye2023mplug2} & 22.7 & 24.9 & 27.2 & 23.9 & 29.7 & 18.8 & 25.2 \\
SPHINX* \cite{lin2023sphinx} & 26.7 & 25.3 & 29.0 & 20.1 & 32.6 & 23.8 & 21.8  \\
Qwen-VL-7B-Chat~\cite{Qwen-VL} & 29.3 & 25.6 & 27.8 & 23.1 & 28.8 & 24.6 & 24.3 \\
Bunny-3B* \cite{Bunny-3B} & 30.7 & 26.8 & 32.8 & 25.2 & 27.8 & 26.5 & 22.8 \\
LLaVA-1.5-13B~\cite{liu2023improved} & 29.3 & 25.9 & 27.2 & 25.0 & 28.8 & 24.0 & 24.5 \\
\bottomrule
\end{tabular}%
\end{adjustbox}
\caption{\textbf{Science} results of different models on the \dataset \textbf{validation} and \textbf{test set}.  The best-performing model in each category is \textbf{in-bold}, and the second best is {\ul{underlined}}. *: results provided by the authors.} 
\label{tab:overall_Science_results}
\end{table*}

\begin{table*}[!t]
\centering
\small
\begin{adjustbox}{scale=0.83}
\begin{tabular}{@{}lcccc|cccc@{}}
\toprule
\textbf{} & \textbf{\begin{tabular}[c]{@{}c@{}}Voice \\ Judge\end{tabular}} & 
\textbf{\begin{tabular}[c]{@{}c@{}}Singing \\ Judge\end{tabular}} & 
\textbf{\begin{tabular}[c]{@{}c@{}}Environment \\ Sound Judge\end{tabular}} & 
\textbf{\begin{tabular}[c]{@{}c@{}}Music \\ Judge\end{tabular}} & 
\textbf{\begin{tabular}[c]{@{}c@{}}Voice \\ Choice\end{tabular}} & 
\textbf{\begin{tabular}[c]{@{}c@{}}Singing \\ Choice\end{tabular}} & 
\textbf{\begin{tabular}[c]{@{}c@{}}Environment \\ Sound Choice\end{tabular}} & 
\textbf{\begin{tabular}[c]{@{}c@{}}Music \\ Choice\end{tabular}}\\ \midrule
\color{Gray} Random Choice & \color{Gray} 22.1 & \color{Gray} 23.9 & \color{Gray} 24.1 & \color{Gray} 24.9 & \color{Gray} 21.6 & \color{Gray} 25.3 & \color{Gray} 22.8 & \color{Gray} 24.8 \\ 
\color{Gray} Frequent Choice & \color{Gray} 26.8 & \color{Gray} 25.8 & \color{Gray} 26.7 & \color{Gray} 28.4 & \color{Gray} 24.0 & \color{Gray} 24.4 & \color{Gray} 25.2 & \color{Gray} 26.5 \\
Expert (Worst)  &76.2 &- &- &- &- &- &- &- \\
Expert (Medium)  &82.6 &- &- &- &- &- &- &- \\
Expert (Best)  &88.6 &- &- &- &- &- &- &- \\
\midrule
% \multicolumn{8}{c}{\textbf{Large Multimodal Models (LMMs): Text + Image as Input}} \\ 
% \midrule
OpenFlamingo2-9B \cite{awadalla2023openflamingo} & 28.7 & 26.3 & 31.7 & 23.5 & 26.3 & 26.3 & 27.9 & 25.1 \\
Kosmos2 \cite{peng2023kosmos} & 24.4 & 26.6 & 28.8 & 23.7 & 26.6 & 27.2 & 26.3 & 26.8 \\
Adept Fuyu-8B~\cite{fuyu-8b} & 27.9 & 27.4 & 29.9 & 27.0 & 25.6 & 27.0 & 32.5 & 26.4 \\
MiniGPT4-Vicuna-13B~\cite{zhu2023minigpt} & 26.8 & 27.6 & 30.2 & 27.0 & 26.2 & 26.9 & 30.9 & 27.2 \\
LLaMA-Adapter2-7B~\cite{zhang2023llama} & 29.8 & 27.7 & 35.2 & 25.4 & 25.6 & 30.0 & 29.1 & 25.7 \\
CogVLM~\cite{COGVLM} & 32.1 & 30.1 & 38.0 & 25.6 & 25.1 & 31.2 & 41.5 & 28.9 \\
Qwen-VL-7B-Chat~\cite{Qwen-VL} & 35.9 & 32.9 & 47.7 & 29.8 & 25.6 & 33.6 & 45.3 & 30.2 \\
InstructBLIP-T5-XXL~\cite{dai2023instructblip} & 35.7 & 33.8 & 48.5 & 30.6 & 27.6 & 33.6 & 49.8 & 29.4 \\
BLIP-2 FLAN-T5-XXL~\cite{li2023blip} & 35.4 & 34.0 & 49.2 & 28.6 & 27.3 & 33.7 & 51.5 & 30.4 \\
InternLM-XComposer2-VL* \cite{dong2024internlm} & 43.0 & 38.2 & 56.8 & 32.8 & 30.1 & 39.8 & 60.7 & 31.8 \\ 
Yi-VL-34B*  \cite{young2024yi} & 45.9 & 41.6 & 56.1 & 33.3 & 32.9 & 45.9 & 66.5 & 36.0 \\
LLaVA-1.6-34B* \cite{liu2024llava} & 51.1 & 44.7 & 58.6 & {\ul 39.9} & 36.0 & {\ul 51.2} & {\ul 70.2} & 36.3 \\
InternVL-Chat-V1.2* \cite{chen2023internvl} & {\ul 51.6} & {\ul 46.2} & \textbf{62.5} & 37.6 & \textbf{37.9} & 49.7 & 70.1 & \textbf{40.8} \\ 
VILA1.5* \cite{lin2023vila} & \textbf{51.9} & \textbf{46.9} & {\ul 62.1} & \textbf{40.6} & {\ul 37.7} & \textbf{51.7} & \textbf{74.0} & {\ul 39.5} \\ \midrule
Qwen-VL-MAX* \cite{Qwen-VL-MAX} & 51.4 & 46.8 & {\ul 64.2} & 39.8 & 36.3 & 52.5 & 70.4 & 40.7 \\
SenseChat-Vision-0423-Preview* \cite{SenseChat-Vision} & 54.6 & {\ul 50.3} & 62.7 & {\ul 44.1} & {\ul 42.3} & {\ul 55.7} & {\ul 74.7} & \textbf{43.5}  \\
GPT-4V(ision) (Playground) \cite{openai2023gpt4v} & 56.8 & \textbf{55.7} & \textbf{65.3} & \textbf{64.3} & \textbf{48.4} & \textbf{63.5} & \textbf{76.3} & {\ul 41.7} \\
Claude 3 Opus* \cite{Claude3} & 59.4 & - & - & - & - & - & - & -  \\
Gemini 1.5 Pro* \cite{deepmind_gemini1.5_report} & {\ul 62.2} & - & - & - & - & - & - & -  \\
GPT-4o* \cite{gpt-4o} & \textbf{69.1} & - & - & - & - & - & - & -  \\  
\bottomrule
\end{tabular}%
\end{adjustbox}
\caption{Selected results of different models on the \dataset \textbf{validation} and \textbf{test set}. Besides reporting the performance of LMMs, we additionally add text-only LLM baselines. The best-performing model in each category is \textbf{in-bold}, and the second best is {\ul{underlined}}. *: results provided by the authors. Due to the page limit, we show other models' results in Appendix \autoref{tab:main_results}. The live-updating leaderboard is available at: \url{https://mmmu-benchmark.github.io/\#leaderboard}}
\label{tab:overall_results}
\end{table*}

\begin{table*}[!t]
\centering
\small
\begin{adjustbox}{scale=0.83}
\begin{tabular}{@{}lcccc|cccc@{}}
\toprule
\textbf{} & \textbf{\begin{tabular}[c]{@{}c@{}}Voice \\ Judge\end{tabular}} & 
\textbf{\begin{tabular}[c]{@{}c@{}}Singing \\ Judge\end{tabular}} & 
\textbf{\begin{tabular}[c]{@{}c@{}}Environment \\ Sound Judge\end{tabular}} & 
\textbf{\begin{tabular}[c]{@{}c@{}}Music \\ Judge\end{tabular}} & 
\textbf{\begin{tabular}[c]{@{}c@{}}Voice \\ Choice\end{tabular}} & 
\textbf{\begin{tabular}[c]{@{}c@{}}Singing \\ Choice\end{tabular}} & 
\textbf{\begin{tabular}[c]{@{}c@{}}Environment \\ Sound Choice\end{tabular}} & 
\textbf{\begin{tabular}[c]{@{}c@{}}Music \\ Choice\end{tabular}}\\ \midrule
\color{Gray} Random Choice & \color{Gray} 22.1 & \color{Gray} 23.9 & \color{Gray} 24.1 & \color{Gray} 24.9 & \color{Gray} 21.6 & \color{Gray} 25.3 & \color{Gray} 22.8 & \color{Gray} 24.8 \\ 
\color{Gray} Frequent Choice & \color{Gray} 26.8 & \color{Gray} 25.8 & \color{Gray} 26.7 & \color{Gray} 28.4 & \color{Gray} 24.0 & \color{Gray} 24.4 & \color{Gray} 25.2 & \color{Gray} 26.5 \\
Expert (Worst)  &76.2 &- &- &- &- &- &- &- \\
Expert (Medium)  &82.6 &- &- &- &- &- &- &- \\
Expert (Best)  &88.6 &- &- &- &- &- &- &- \\
\midrule
% \multicolumn{8}{c}{\textbf{Large Multimodal Models (LMMs): Text + Image as Input}} \\ 
% \midrule
OpenFlamingo2-9B \cite{awadalla2023openflamingo} & 28.7 & 26.3 & 31.7 & 23.5 & 26.3 & 26.3 & 27.9 & 25.1 \\
Kosmos2 \cite{peng2023kosmos} & 24.4 & 26.6 & 28.8 & 23.7 & 26.6 & 27.2 & 26.3 & 26.8 \\
Adept Fuyu-8B~\cite{fuyu-8b} & 27.9 & 27.4 & 29.9 & 27.0 & 25.6 & 27.0 & 32.5 & 26.4 \\
MiniGPT4-Vicuna-13B~\cite{zhu2023minigpt} & 26.8 & 27.6 & 30.2 & 27.0 & 26.2 & 26.9 & 30.9 & 27.2 \\
LLaMA-Adapter2-7B~\cite{zhang2023llama} & 29.8 & 27.7 & 35.2 & 25.4 & 25.6 & 30.0 & 29.1 & 25.7 \\
CogVLM~\cite{COGVLM} & 32.1 & 30.1 & 38.0 & 25.6 & 25.1 & 31.2 & 41.5 & 28.9 \\
Qwen-VL-7B-Chat~\cite{Qwen-VL} & 35.9 & 32.9 & 47.7 & 29.8 & 25.6 & 33.6 & 45.3 & 30.2 \\
InstructBLIP-T5-XXL~\cite{dai2023instructblip} & 35.7 & 33.8 & 48.5 & 30.6 & 27.6 & 33.6 & 49.8 & 29.4 \\
BLIP-2 FLAN-T5-XXL~\cite{li2023blip} & 35.4 & 34.0 & 49.2 & 28.6 & 27.3 & 33.7 & 51.5 & 30.4 \\
InternLM-XComposer2-VL* \cite{dong2024internlm} & 43.0 & 38.2 & 56.8 & 32.8 & 30.1 & 39.8 & 60.7 & 31.8 \\ 
Yi-VL-34B*  \cite{young2024yi} & 45.9 & 41.6 & 56.1 & 33.3 & 32.9 & 45.9 & 66.5 & 36.0 \\
LLaVA-1.6-34B* \cite{liu2024llava} & 51.1 & 44.7 & 58.6 & {\ul 39.9} & 36.0 & {\ul 51.2} & {\ul 70.2} & 36.3 \\
InternVL-Chat-V1.2* \cite{chen2023internvl} & {\ul 51.6} & {\ul 46.2} & \textbf{62.5} & 37.6 & \textbf{37.9} & 49.7 & 70.1 & \textbf{40.8} \\ 
VILA1.5* \cite{lin2023vila} & \textbf{51.9} & \textbf{46.9} & {\ul 62.1} & \textbf{40.6} & {\ul 37.7} & \textbf{51.7} & \textbf{74.0} & {\ul 39.5} \\ \midrule
Qwen-VL-MAX* \cite{Qwen-VL-MAX} & 51.4 & 46.8 & {\ul 64.2} & 39.8 & 36.3 & 52.5 & 70.4 & 40.7 \\
SenseChat-Vision-0423-Preview* \cite{SenseChat-Vision} & 54.6 & {\ul 50.3} & 62.7 & {\ul 44.1} & {\ul 42.3} & {\ul 55.7} & {\ul 74.7} & \textbf{43.5}  \\
GPT-4V(ision) (Playground) \cite{openai2023gpt4v} & 56.8 & \textbf{55.7} & \textbf{65.3} & \textbf{64.3} & \textbf{48.4} & \textbf{63.5} & \textbf{76.3} & {\ul 41.7} \\
Claude 3 Opus* \cite{Claude3} & 59.4 & - & - & - & - & - & - & -  \\
Gemini 1.5 Pro* \cite{deepmind_gemini1.5_report} & {\ul 62.2} & - & - & - & - & - & - & -  \\
GPT-4o* \cite{gpt-4o} & \textbf{69.1} & - & - & - & - & - & - & -  \\  
\bottomrule
\end{tabular}%
\end{adjustbox}
\caption{Selected results of different models on the \dataset \textbf{validation} and \textbf{test set}. Besides reporting the performance of LMMs, we additionally add text-only LLM baselines. The best-performing model in each category is \textbf{in-bold}, and the second best is {\ul{underlined}}. *: results provided by the authors. Due to the page limit, we show other models' results in Appendix \autoref{tab:main_results}. The live-updating leaderboard is available at: \url{https://mmmu-benchmark.github.io/\#leaderboard}}
\label{tab:overall_results}
\end{table*}

\begin{table*}[!b]
\centering
\small
\begin{adjustbox}{scale = 0.8}
\begin{tabular}{@{}lcccccc@{}}
\toprule
\textbf{} & \textbf{\begin{tabular}[c]{@{}c@{}}Nerf \\ Judge\end{tabular}} & \textbf{\begin{tabular}[c]{@{}c@{}}Gaussian \\ Judge\end{tabular}} & \textbf{\begin{tabular}[c]{@{}c@{}}Others \\ Judge\end{tabular}} & \textbf{\begin{tabular}[c]{@{}c@{}}Nerf \\ Choice\end{tabular}} & \textbf{\begin{tabular}[c]{@{}c@{}}Gaussian \\ Choice\end{tabular}} & \textbf{\begin{tabular}[c]{@{}c@{}}Others \\ Choice\end{tabular}} \\ \midrule

\color{Gray} Random Choice & \color{Gray} 18.0 & \color{Gray} 21.6 & \color{Gray} 18.3 & \color{Gray} 18.6 & \color{Gray} 26.0 & \color{Gray} 22.2\\   
\color{Gray} Frequent Choice & \color{Gray} 27.3 & \color{Gray} 24.0 & \color{Gray} 25.8 & \color{Gray} 19.9 & \color{Gray} 26.9 & \color{Gray} 26.1\\
Expert (Worst)  & 78.0 & - & - & - & - & - \\
Expert (Medium)  & 84.7 & - & - & - & - & - \\
Expert (Best)  & 90.0 & - & - & - & - & - \\
\midrule
OpenFlamingo2-9B \cite{awadalla2023openflamingo} & 23.3 & 26.3 & 27.8 & 22.9 & 30.8 & 25.1 \\
Kosmos2 \cite{peng2023kosmos} & 19.3 & 26.6 & 28.4 & 21.7 & 29.2 & 26.7 \\
Fuyu-8B~\cite{fuyu-8b} & 22.0 & 25.6 & 27.8 & 20.9 & 30.1 & 24.8 \\
MiniGPT4-Vicuna-13B~\cite{zhu2023minigpt} & 28.7 & 26.2 & 23.2 & 22.1 & 29.4 & 30.1 \\
LLaMA-Adapter2-7B~\cite{zhang2023llama} & 30.7 & 25.6 & 27.5 & 24.9 & 30.4 & 23.0 \\
Otter~\cite{li2023otter} & 34.7 & 24.1 & 24.6 & 23.4 & 27.1 & 23.0 \\
CogVLM~\cite{COGVLM} & 28.0 & 25.1 & 29.3 & 24.2 & 28.0 & 23.4 \\
InstructBLIP-T5-XL~\cite{dai2023instructblip} & 32.7 & 25.2 & 27.0 & 22.1 & 28.3 & 24.4 \\
BLIP-2 FLAN-T5-XL \cite{li2023blip} & 30.7 & 25.1 & 26.7 & 24.4 & 25.7 & 24.0 \\
mPLUG-OWL2* \cite{ye2023mplug2} & 22.7 & 24.9 & 27.2 & 23.9 & 29.7 & 18.8 \\
SPHINX* \cite{lin2023sphinx} & 26.7 & 25.3 & 29.0 & 20.1 & 32.6 & 23.8  \\
Qwen-VL-7B-Chat~\cite{Qwen-VL} & 29.3 & 25.6 & 27.8 & 23.1 & 28.8 & 24.6 \\
Bunny-3B* \cite{Bunny-3B} & 30.7 & 26.8 & 32.8 & 25.2 & 27.8 & 26.5 \\
LLaVA-1.5-13B~\cite{liu2023improved} & 29.3 & 25.9 & 27.2 & 25.0 & 28.8 & 24.0 \\
\bottomrule
\end{tabular}
\end{adjustbox}
\caption{3D} 
\label{tab:overall_Science_results}
\end{table*}

\begin{table*}[!t]
\centering
\small
\begin{adjustbox}{scale=0.83}
\begin{tabular}{@{}lcccccccc@{}}
\toprule
\textbf{} & \textbf{\begin{tabular}[c]{@{}c@{}}Scientific\\Papers \end{tabular}} & 
\textbf{\begin{tabular}[c]{@{}c@{}}News \end{tabular}} & 
\textbf{\begin{tabular}[c]{@{}c@{}}Essay \end{tabular}} & 
\textbf{\begin{tabular}[c]{@{}c@{}}Wikipedia \end{tabular}} & 
\textbf{\begin{tabular}[c]{@{}c@{}}Speech \end{tabular}} & 
\textbf{\begin{tabular}[c]{@{}c@{}}Modern \\ Literature \end{tabular}} & 
\textbf{\begin{tabular}[c]{@{}c@{}}Phiosophy \end{tabular}} & 
\textbf{\begin{tabular}[c]{@{}c@{}}Ancient  Chinese\end{tabular}}\\ \midrule
\color{Gray} Random Choice & \color{Gray} 22.1 & \color{Gray} 23.9 & \color{Gray} 24.1 & \color{Gray} 24.9 & \color{Gray} 21.6 & \color{Gray} 25.3 & \color{Gray} 22.8 & \color{Gray} 24.8 \\ 
\color{Gray} Frequent Choice & \color{Gray} 26.8 & \color{Gray} 25.8 & \color{Gray} 26.7 & \color{Gray} 28.4 & \color{Gray} 24.0 & \color{Gray} 24.4 & \color{Gray} 25.2 & \color{Gray} 26.5 \\
Expert (Worst)  &76.2 &- &- &- &- &- &- &- \\
Expert (Medium)  &82.6 &- &- &- &- &- &- &- \\
Expert (Best)  &88.6 &- &- &- &- &- &- &- \\
\midrule
% \multicolumn{8}{c}{\textbf{Large Multimodal Models (LMMs): Text + Image as Input}} \\ 
% \midrule
OpenFlamingo2-9B \cite{awadalla2023openflamingo} & 28.7 & 26.3 & 31.7 & 23.5 & 26.3 & 26.3 & 27.9 & 25.1 \\
Kosmos2 \cite{peng2023kosmos} & 24.4 & 26.6 & 28.8 & 23.7 & 26.6 & 27.2 & 26.3 & 26.8 \\
Adept Fuyu-8B~\cite{fuyu-8b} & 27.9 & 27.4 & 29.9 & 27.0 & 25.6 & 27.0 & 32.5 & 26.4 \\
MiniGPT4-Vicuna-13B~\cite{zhu2023minigpt} & 26.8 & 27.6 & 30.2 & 27.0 & 26.2 & 26.9 & 30.9 & 27.2 \\
LLaMA-Adapter2-7B~\cite{zhang2023llama} & 29.8 & 27.7 & 35.2 & 25.4 & 25.6 & 30.0 & 29.1 & 25.7 \\
CogVLM~\cite{COGVLM} & 32.1 & 30.1 & 38.0 & 25.6 & 25.1 & 31.2 & 41.5 & 28.9 \\
Qwen-VL-7B-Chat~\cite{Qwen-VL} & 35.9 & 32.9 & 47.7 & 29.8 & 25.6 & 33.6 & 45.3 & 30.2 \\
InstructBLIP-T5-XXL~\cite{dai2023instructblip} & 35.7 & 33.8 & 48.5 & 30.6 & 27.6 & 33.6 & 49.8 & 29.4 \\
BLIP-2 FLAN-T5-XXL~\cite{li2023blip} & 35.4 & 34.0 & 49.2 & 28.6 & 27.3 & 33.7 & 51.5 & 30.4 \\
InternLM-XComposer2-VL* \cite{dong2024internlm} & 43.0 & 38.2 & 56.8 & 32.8 & 30.1 & 39.8 & 60.7 & 31.8 \\ 
Yi-VL-34B*  \cite{young2024yi} & 45.9 & 41.6 & 56.1 & 33.3 & 32.9 & 45.9 & 66.5 & 36.0 \\
LLaVA-1.6-34B* \cite{liu2024llava} & 51.1 & 44.7 & 58.6 & {\ul 39.9} & 36.0 & {\ul 51.2} & {\ul 70.2} & 36.3 \\
InternVL-Chat-V1.2* \cite{chen2023internvl} & {\ul 51.6} & {\ul 46.2} & \textbf{62.5} & 37.6 & \textbf{37.9} & 49.7 & 70.1 & \textbf{40.8} \\ 
VILA1.5* \cite{lin2023vila} & \textbf{51.9} & \textbf{46.9} & {\ul 62.1} & \textbf{40.6} & {\ul 37.7} & \textbf{51.7} & \textbf{74.0} & {\ul 39.5} \\ \midrule
Qwen-VL-MAX* \cite{Qwen-VL-MAX} & 51.4 & 46.8 & {\ul 64.2} & 39.8 & 36.3 & 52.5 & 70.4 & 40.7 \\
SenseChat-Vision-0423-Preview* \cite{SenseChat-Vision} & 54.6 & {\ul 50.3} & 62.7 & {\ul 44.1} & {\ul 42.3} & {\ul 55.7} & {\ul 74.7} & \textbf{43.5}  \\
GPT-4V(ision) (Playground) \cite{openai2023gpt4v} & 56.8 & \textbf{55.7} & \textbf{65.3} & \textbf{64.3} & \textbf{48.4} & \textbf{63.5} & \textbf{76.3} & {\ul 41.7} \\
Claude 3 Opus* \cite{Claude3} & 59.4 & - & - & - & - & - & - & -  \\
Gemini 1.5 Pro* \cite{deepmind_gemini1.5_report} & {\ul 62.2} & - & - & - & - & - & - & -  \\
GPT-4o* \cite{gpt-4o} & \textbf{69.1} & - & - & - & - & - & - & -  \\  
\bottomrule
\end{tabular}%
\end{adjustbox}
\caption{Selected results of different models on the \dataset \textbf{validation} and \textbf{test set}. Besides reporting the performance of LMMs, we additionally add text-only LLM baselines. The best-performing model in each category is \textbf{in-bold}, and the second best is {\ul{underlined}}. *: results provided by the authors. Due to the page limit, we show other models' results in Appendix \autoref{tab:main_results}. The live-updating leaderboard is available at: \url{https://mmmu-benchmark.github.io/\#leaderboard}}
\label{tab:overall_results}
\end{table*}

\begin{table*}[!t]
\centering
\small
\begin{adjustbox}{scale=0.83}
\begin{tabular}{@{}lcccccccc@{}}
\toprule
\textbf{} & \textbf{\begin{tabular}[c]{@{}c@{}}Scientific\\Papers \end{tabular}} & 
\textbf{\begin{tabular}[c]{@{}c@{}}News \end{tabular}} & 
\textbf{\begin{tabular}[c]{@{}c@{}}Essay \end{tabular}} & 
\textbf{\begin{tabular}[c]{@{}c@{}}Wikipedia \end{tabular}} & 
\textbf{\begin{tabular}[c]{@{}c@{}}Speech \end{tabular}} & 
\textbf{\begin{tabular}[c]{@{}c@{}}Modern \\ Literature \end{tabular}} & 
\textbf{\begin{tabular}[c]{@{}c@{}}Phiosophy \end{tabular}} & 
\textbf{\begin{tabular}[c]{@{}c@{}}Ancient  Chinese\end{tabular}}\\ \midrule
\color{Gray} Random Choice & \color{Gray} 22.1 & \color{Gray} 23.9 & \color{Gray} 24.1 & \color{Gray} 24.9 & \color{Gray} 21.6 & \color{Gray} 25.3 & \color{Gray} 22.8 & \color{Gray} 24.8 \\ 
\color{Gray} Frequent Choice & \color{Gray} 26.8 & \color{Gray} 25.8 & \color{Gray} 26.7 & \color{Gray} 28.4 & \color{Gray} 24.0 & \color{Gray} 24.4 & \color{Gray} 25.2 & \color{Gray} 26.5 \\
Expert (Worst)  &76.2 &- &- &- &- &- &- &- \\
Expert (Medium)  &82.6 &- &- &- &- &- &- &- \\
Expert (Best)  &88.6 &- &- &- &- &- &- &- \\
\midrule
% \multicolumn{8}{c}{\textbf{Large Multimodal Models (LMMs): Text + Image as Input}} \\ 
% \midrule
OpenFlamingo2-9B \cite{awadalla2023openflamingo} & 28.7 & 26.3 & 31.7 & 23.5 & 26.3 & 26.3 & 27.9 & 25.1 \\
Kosmos2 \cite{peng2023kosmos} & 24.4 & 26.6 & 28.8 & 23.7 & 26.6 & 27.2 & 26.3 & 26.8 \\
Adept Fuyu-8B~\cite{fuyu-8b} & 27.9 & 27.4 & 29.9 & 27.0 & 25.6 & 27.0 & 32.5 & 26.4 \\
MiniGPT4-Vicuna-13B~\cite{zhu2023minigpt} & 26.8 & 27.6 & 30.2 & 27.0 & 26.2 & 26.9 & 30.9 & 27.2 \\
LLaMA-Adapter2-7B~\cite{zhang2023llama} & 29.8 & 27.7 & 35.2 & 25.4 & 25.6 & 30.0 & 29.1 & 25.7 \\
CogVLM~\cite{COGVLM} & 32.1 & 30.1 & 38.0 & 25.6 & 25.1 & 31.2 & 41.5 & 28.9 \\
Qwen-VL-7B-Chat~\cite{Qwen-VL} & 35.9 & 32.9 & 47.7 & 29.8 & 25.6 & 33.6 & 45.3 & 30.2 \\
InstructBLIP-T5-XXL~\cite{dai2023instructblip} & 35.7 & 33.8 & 48.5 & 30.6 & 27.6 & 33.6 & 49.8 & 29.4 \\
BLIP-2 FLAN-T5-XXL~\cite{li2023blip} & 35.4 & 34.0 & 49.2 & 28.6 & 27.3 & 33.7 & 51.5 & 30.4 \\
InternLM-XComposer2-VL* \cite{dong2024internlm} & 43.0 & 38.2 & 56.8 & 32.8 & 30.1 & 39.8 & 60.7 & 31.8 \\ 
Yi-VL-34B*  \cite{young2024yi} & 45.9 & 41.6 & 56.1 & 33.3 & 32.9 & 45.9 & 66.5 & 36.0 \\
LLaVA-1.6-34B* \cite{liu2024llava} & 51.1 & 44.7 & 58.6 & {\ul 39.9} & 36.0 & {\ul 51.2} & {\ul 70.2} & 36.3 \\
InternVL-Chat-V1.2* \cite{chen2023internvl} & {\ul 51.6} & {\ul 46.2} & \textbf{62.5} & 37.6 & \textbf{37.9} & 49.7 & 70.1 & \textbf{40.8} \\ 
VILA1.5* \cite{lin2023vila} & \textbf{51.9} & \textbf{46.9} & {\ul 62.1} & \textbf{40.6} & {\ul 37.7} & \textbf{51.7} & \textbf{74.0} & {\ul 39.5} \\ \midrule
Qwen-VL-MAX* \cite{Qwen-VL-MAX} & 51.4 & 46.8 & {\ul 64.2} & 39.8 & 36.3 & 52.5 & 70.4 & 40.7 \\
SenseChat-Vision-0423-Preview* \cite{SenseChat-Vision} & 54.6 & {\ul 50.3} & 62.7 & {\ul 44.1} & {\ul 42.3} & {\ul 55.7} & {\ul 74.7} & \textbf{43.5}  \\
GPT-4V(ision) (Playground) \cite{openai2023gpt4v} & 56.8 & \textbf{55.7} & \textbf{65.3} & \textbf{64.3} & \textbf{48.4} & \textbf{63.5} & \textbf{76.3} & {\ul 41.7} \\
Claude 3 Opus* \cite{Claude3} & 59.4 & - & - & - & - & - & - & -  \\
Gemini 1.5 Pro* \cite{deepmind_gemini1.5_report} & {\ul 62.2} & - & - & - & - & - & - & -  \\
GPT-4o* \cite{gpt-4o} & \textbf{69.1} & - & - & - & - & - & - & -  \\  
\bottomrule
\end{tabular}%
\end{adjustbox}
\caption{Selected results of different models on the \dataset \textbf{validation} and \textbf{test set}. Besides reporting the performance of LMMs, we additionally add text-only LLM baselines. The best-performing model in each category is \textbf{in-bold}, and the second best is {\ul{underlined}}. *: results provided by the authors. Due to the page limit, we show other models' results in Appendix \autoref{tab:main_results}. The live-updating leaderboard is available at: \url{https://mmmu-benchmark.github.io/\#leaderboard}}
\label{tab:overall_results}
\end{table*}

\setlength{\tabcolsep}{8pt}

\resizebox{0.95\textwidth}{!}{%
\begin{tabular}{@{}ccccc@{}}
\toprule
\textbf{Model Family} & \textbf{Model Version} & \textbf{Parameters} & \textbf{Model Type} & \textbf{Parallel Type} \\ \midrule
\multicolumn{1}{c|}{\multirow{2}{*}{InstructBLIP}} & \multicolumn{1}{c|}{InstructBLIP-Vicuna-7B} & \multicolumn{1}{c|}{7B} & \multicolumn{1}{c|}{Open-sourced} & Data \\
\multicolumn{1}{c|}{} & \multicolumn{1}{c|}{InstructBLIP-Vicuna-13B} & \multicolumn{1}{c|}{13B} & \multicolumn{1}{c|}{Open-sourced} & Data \\ \midrule
\multicolumn{1}{c|}{Fuyu} & \multicolumn{1}{c|}{Fuyu-8B} & \multicolumn{1}{c|}{8B} & \multicolumn{1}{c|}{Open-sourced} & Data \\ 
\multicolumn{1}{c|}{Idefics} & \multicolumn{1}{c|}{Idefics-2-8B} & \multicolumn{1}{c|}{8B} & \multicolumn{1}{c|}{Open-sourced} & Data \\ 
\multicolumn{1}{c|}{MiniCPM} & \multicolumn{1}{c|}{MiniCPM-V 2.8B} & \multicolumn{1}{c|}{2.8B} & \multicolumn{1}{c|}{Open-sourced} & Data \\ 
\multicolumn{1}{c|}{XComposer} & \multicolumn{1}{c|}{XComposer-4KHD} & \multicolumn{1}{c|}{8B} & \multicolumn{1}{c|}{Open-sourced} & Data \\ 
\multicolumn{1}{c|}{InternVL} & \multicolumn{1}{c|}{InternVL-1.5} & \multicolumn{1}{c|}{26B} & \multicolumn{1}{c|}{Open-sourced} & Data \\ \midrule
\multicolumn{1}{c|}{\multirow{9}{*}{LLaVA}} & \multicolumn{1}{c|}{LLaVA-1.5-7B} & \multicolumn{1}{c|}{7B} & \multicolumn{1}{c|}{Open-sourced} & Data \\
\multicolumn{1}{c|}{} & \multicolumn{1}{c|}{LLaVA-1.5-13B} & \multicolumn{1}{c|}{13B} & \multicolumn{1}{c|}{Open-sourced} & Data \\
\multicolumn{1}{c|}{} & \multicolumn{1}{c|}{LLaVA-NeXT-Vicuna-7B} & \multicolumn{1}{c|}{7B} & \multicolumn{1}{c|}{Open-sourced} & Data \\
\multicolumn{1}{c|}{} & \multicolumn{1}{c|}{LLaVA-NeXT-Vicuna-13B} & \multicolumn{1}{c|}{13B} & \multicolumn{1}{c|}{Open-sourced} & Data \\
\multicolumn{1}{c|}{} & \multicolumn{1}{c|}{LLaVA-NeXT-Mistral-7B} & \multicolumn{1}{c|}{7B} & \multicolumn{1}{c|}{Open-sourced} & Data \\
\multicolumn{1}{c|}{} & \multicolumn{1}{c|}{LLaVA-NeXT-Yi-34B} & \multicolumn{1}{c|}{34B} & \multicolumn{1}{c|}{Open-sourced} & Data \\
\multicolumn{1}{c|}{} & \multicolumn{1}{c|}{LLaVA-NeXT-LLaMA-3-8B} & \multicolumn{1}{c|}{8B} & \multicolumn{1}{c|}{Open-sourced} & Data \\
\multicolumn{1}{c|}{} & \multicolumn{1}{c|}{LLaVA-NeXT-Qwen-72B} & \multicolumn{1}{c|}{72B} & \multicolumn{1}{c|}{Open-sourced} & Model \\
\multicolumn{1}{c|}{} & \multicolumn{1}{c|}{LLaVA-NeXT-Qwen-110B} & \multicolumn{1}{c|}{110B} & \multicolumn{1}{c|}{Open-sourced} & Model \\ \midrule
\multicolumn{1}{c|}{\multirow{3}{*}{Qwen-VL}} & \multicolumn{1}{c|}{Qwen-VL-Chat-7B} & \multicolumn{1}{c|}{7B} & \multicolumn{1}{c|}{Open-sourced} & Data \\
\multicolumn{1}{c|}{} & \multicolumn{1}{c|}{Qwen-VL-Plus} & \multicolumn{1}{c|}{N/A} & \multicolumn{1}{c|}{Close-sourced, API} & Data \\
\multicolumn{1}{c|}{} & \multicolumn{1}{c|}{Qwen-VL-MAX} & \multicolumn{1}{c|}{N/A} & \multicolumn{1}{c|}{Close-sourced, API} & Data \\ \midrule
\multicolumn{1}{c|}{\multirow{3}{*}{Gemini}} & \multicolumn{1}{c|}{Gemini-1.0-Pro} & \multicolumn{1}{c|}{N/A} & \multicolumn{1}{c|}{Close-sourced, API} & Data \\
\multicolumn{1}{c|}{} & \multicolumn{1}{c|}{Gemini-1.5-Flash} & \multicolumn{1}{c|}{N/A} & \multicolumn{1}{c|}{Close-sourced, API} & Data \\
\multicolumn{1}{c|}{} & \multicolumn{1}{c|}{Gemini-1.5-Pro} & \multicolumn{1}{c|}{N/A} & \multicolumn{1}{c|}{Close-sourced, API} & Data \\ \midrule
\multicolumn{1}{c|}{\multirow{2}{*}{GPT4}} & \multicolumn{1}{c|}{GPT-4V} & \multicolumn{1}{c|}{N/A} & \multicolumn{1}{c|}{Close-sourced, API} & Data \\
\multicolumn{1}{c|}{} & \multicolumn{1}{c|}{GPT-4O} & \multicolumn{1}{c|}{N/A} & \multicolumn{1}{c|}{Close-sourced, API} & Data \\ \midrule
\multicolumn{1}{c|}{\multirow{3}{*}{Claude}} & \multicolumn{1}{c|}{Claude-3-Haku} & \multicolumn{1}{c|}{N/A} & \multicolumn{1}{c|}{Close-sourced, API} & Data \\
\multicolumn{1}{c|}{} & \multicolumn{1}{c|}{Claude-3-Sonnet} & \multicolumn{1}{c|}{N/A} & \multicolumn{1}{c|}{Close-sourced, API} & Data \\
\multicolumn{1}{c|}{} & \multicolumn{1}{c|}{Claude-3-Opus} & \multicolumn{1}{c|}{N/A} & \multicolumn{1}{c|}{Close-sourced, API} & Data \\ \bottomrule
\end{tabular}%
}
